# Supplementary material for: Solvable Strong-coupling Quantum Dot Model with a Non-Fermi-liquid Pairing Transition
Source: arXiv:1904.07240 ancillary file (2020-01-01)
Supplement: Supplementary file 1 [file suppl.pdf]

# Supplemental Material for "Solvable Strong-coupling Quantum Dot Model with a Non-Fermi-liquid Pairing Transition"

Yuxuan Wang[1,2]

[1]Department of Physics, University of Florida, 2001 Museum Rd, Gainesville, FL 32611 USA

[2]Department of Physics, Stanford University, Stanford, CA 94305, USA

(Dated: December 12, 2019)

## I. A DISORDER-FREE MODEL

Much like the SYK model, disorder is not a crucial element for the theory, at least for the normal state. One can consider a disorder-free model similar to the tensor SYK model as follows

$$H = \frac{J}{\sqrt{N}} \sum_{ij}^{N} \sum_{\alpha}^{M} \phi_{ij} c^{\dagger}_{i\alpha} c_{j\alpha} + \sum_{ij}^{N} \left( \frac{1}{2}\pi_{ij}^2 + \frac{m_0^2}{2}\phi_{ij}^2 \right). \tag{1}$$

Despite having no disorder, the diagrams for self-energies are exactly the same type as those in the main text. This is due to the structure of the indices the field carries. As a result, normal state results for this model are very similar to that analyzed in the main text. However, the pairing behavior of this model is different, and in particular the pairing susceptibility is not suppressed by $1/N$.

## II. NORMAL-STATE ANALYSIS FOR A GENERIC BOSON BARE MASS

In the main text we analyzed the normal state self-energy for both weak ($\omega_0 \ll m_0$) and strong ($\omega_0 \gg m_0$) coupling cases at the lowest energies, and showed that strikingly the systems always "self-tunes" to a critical phase, and the nFL behavior persists at the lowest energy scale.[1] In this section we analyze the self-energies at higher frequencies. See also Ref. 2 for details on a related calculation.

### A. Weak coupling case with $\omega_0 \ll m_0$

As we showed in the main text, the nFL energy scale $\omega_F$ is given by the mass renormalization condition,

$$m_0^2 = -\Pi(0) \sim \omega_0^3 \int_{\omega_F} \frac{d\omega}{\omega^2} = \frac{\omega_0^3}{\omega_F}. \tag{2}$$

Thus

$$\omega_F = \frac{\omega_0^3}{m_0^2}. \tag{3}$$

For $\omega, \Omega \gg \omega_F$, the fermionic self-energy is dominated by low-energy bosons

$$\Sigma(\omega) \approx \int_{-\omega_F}^{\omega_F} \frac{d\Omega}{2\pi} \frac{-\omega_0^3}{m_0^2 |\Omega/\omega_F|^{1-2x}} \frac{1}{i\omega} \sim \frac{i\omega_F^2}{\omega} \ll i\omega, \tag{4}$$

and the renormalized boson mass is dominated by its bare form:

$$\tilde{\Pi}(\Omega) \sim m_0^2 - \int_{\Omega} \frac{\omega_0^3 d\omega}{\omega^2} \approx m_0^2. \tag{5}$$

Indeed, the boson and fermion propagators are approximately their bare form, which justifies Eq. (2).

### B. Strong coupling case with $\omega_0 \gg m_0$

As we showed in the main text, in this case the characteristic energy $\omega_B$ for the boson determines the scale up to which low-energy physics persists.

For fermions with $\omega \gg \omega_B$, the boson is essentially static, and the fermionic self-energy has the same behavior as disordered fermions:

$$\Sigma(\omega) = -\frac{\omega_0^3}{\Sigma(\omega)} \int \frac{d\Omega}{\Omega^2 + \tilde{\Pi}(\Omega)} \sim -\frac{\omega_0^3}{\Sigma(\omega)} \frac{1}{\omega_B} \tag{6}$$

Hence

$$\Sigma(\omega) = i\sqrt{\frac{\omega_0^3}{\omega_B}}\, \mathrm{sgn}(\omega). \tag{7}$$

As long as $\omega < \sqrt{\omega_0^3/\omega_B}$, the self-energy still dominates the fermion Green's function, and the fermions still behave as a nFL. The scale $\sqrt{\omega_0^3/\omega_B}$ now serves as the IR cutoff for the bosonic mass renormalization. We have

$$m_0^2 \sim \omega_0^3 \int_{\sqrt{\omega_0^3/\omega_B}} \frac{d\omega}{\omega^2}, \tag{8}$$

and therefore

$$\omega_B = \frac{m_0^4}{\omega_0^3}, \tag{9}$$

The bosonic self-energy in this region $\omega_B \ll \Omega \ll \sqrt{\omega_0^3/\omega_B}$ is then given by

$$\begin{aligned} \tilde{\Pi}(\Omega) \sim & \frac{\omega_0^3}{\omega_0^3/\omega_B} \int d\omega\, \mathrm{sgn}(\omega)\, \mathrm{sgn}(\omega + \Omega) \\ \sim & \omega_B |\Omega|. \end{aligned} \tag{10}$$

For $(\omega, \Omega) > \sqrt{\omega_0^3/\omega_B}$, the fermionic self-energy still resembles that in a disorder problem, only now $\Sigma(\omega) \ll \omega$. The renormalized bosonic mass retains its bare value. We have

$$\begin{aligned} \Sigma(\omega) \sim & i \frac{\omega_0^3}{\omega_B \omega}, \\ \tilde{\Pi}(\Omega) \sim & \frac{\omega_0^3}{\omega_F} \equiv m_0^2. \end{aligned} \tag{11}$$

One can verify that the behaviors of $\Sigma$ and $\tilde{\Pi}$ indeed match at $(\omega, \Omega) \sim \sqrt{\omega_0^3/\omega_B}$.

## III. RENOMALIZTION GROUP FORMULATION OF THE PAIRING PROBLEM

We now reformulate the results on pairing QCP within the renormalization-group (RG) framework. It turns out that there is a direct correspondence[3] between the Eliashberg gap equation and the $\beta$-function of the BCS coupling constant (which needs to be carefully defined for critical interactions). Here we follow the procedure similar to that adopted in Refs. 4 and 5.

The central question we consider is how the four-fermion interaction

$$\begin{aligned} S_{\text{int}} = & - \int d\omega d\omega' d\delta\omega \sum_{ij,\alpha\beta} t^2 D(\omega - \omega') \\ & \times c^\dagger_{j\beta}(\omega) c^\dagger_{i\alpha}(-\omega + \delta\omega) c_{i\alpha}(\omega') c_{j\beta}(-\omega' + \delta\omega), \end{aligned} \tag{12}$$

gets renormalized in the BCS channel ($\delta\omega \sim 0$) under the RG flow. Notice that unlike the usual RG analysis for pairing, the BCS coupling "constant" $t^2 D$ strongly depends on frequency transfer $\Omega \equiv \omega - \omega'$. At any RG time,

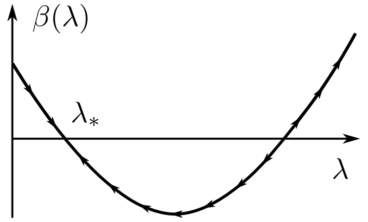


FIG. 1. The $\beta$-function of the BCS coupling constant $\lambda$.

$D(\Omega \to 0) \sim 1/0^{1-2x}$ is always divergent. But clearly this doesn't mean already at UV scale pairing develops. In the gap equation of the main text one integrates over frequency transfer and the integration is convergent. The characteristic scale for the frequency transfer is then the same as that for fermions

$$\Omega \sim \omega \sim \omega'. \tag{13}$$

We then identify an effective BCS coupling constant (let us set $c$ in the main text to 1)

$$\lambda_0(\mu) \equiv \frac{t^2}{\omega_0} D(\bar{c}\mu) = \frac{\omega_0^{1-2x}}{\alpha(x)(\bar{c}\mu)^{1-2x}}, \tag{14}$$

and take $\lambda_0$ as the bare BCS coupling at RG scale[6] $\mu = \omega_0 e^{-\ell}$, where $\bar{c}$ is a non-universal $O(1)$ constant because Eq. (13) is up to a constant. In the above we have used $t^2/\omega_0 = \omega_0^2/g$. This constant factor is added to simplify the one-loop contribution to the RG flow.

We compute the $\beta$-function of the BCS coupling. There are three effects at play here. First, due to the explicit $\mu$ dependence of $\lambda_0$ we have

$$\frac{d\lambda_0}{d\ell} = \frac{1-2x}{\alpha(x)\bar{c}^{1-2x}}, \tag{15}$$

i.e., there is a "tree-level running" of the BCS coupling[7,8]. Unlike conventional contributions to the $\beta$-function from loop diagrams, the tree-level running of $\lambda$ comes from the attractive interaction mediated by a gapless boson, which is singular in frequency. Second, due to the nFL self energy, the fermionic field has the anomalous scaling

$$[c^\dagger(\omega)] = -1/2 - x/2. \tag{16}$$

From Eq. (12), instead of being marginal, the BCS coupling $\lambda$ is irrelevant at tree level with

$$[\lambda] = -(1-2x). \tag{17}$$

Third, at one-loop level $\sim \lambda^2$, the ladder diagram gives a positive contribution to $\beta$-function, just like the RG flow in the conventional BCS theory. Combining these, the $\beta$-function is given by

$$\beta(\lambda) = \frac{d\lambda}{d\ell} = \frac{1-2x}{\alpha(x)\bar{c}^{1-2x}} - (1-2x)\lambda + \frac{\lambda^2}{\pi M}, \tag{18}$$

where the three terms correspond to the three effects described above. We show such an RG flow in Fig. 1. At the cost of an unknown $O(1)$ constant $\bar{c}$, the interplay between the singular attractive interaction and nFL behavior is intuitively encoded in the differential equation. In general the equivalence of the RG approach and the Eliashberg equation approach can be established by converting the latter from an integral equation to a differential equation, as was shown explicitly in Ref. 3.

A simple analysis of Eq (18) shows that for $M < 8/[\alpha(x)\bar{c}^{1-2x}(1-2x)]$, $\lambda$ flows to infinity and correspondingly the system enters a pairing phase. On the other hand, if

$$M > \frac{4}{\pi\alpha(x)\bar{c}^{1-2x}(1-2x)}, \tag{19}$$

there exists a *stable* fixed point at (see Fig. 1)

$$\lambda_* = \frac{(1-2x) - \sqrt{(1-2x)^2 - 4(1-2x)/(\pi\alpha M\bar{c}^{1-2x})}}{2/(\pi M)}, \tag{20}$$

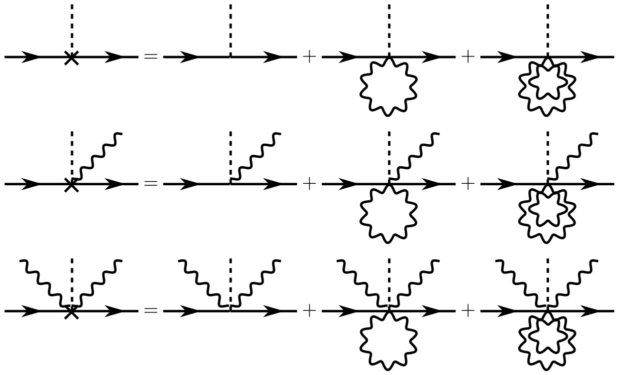

FIG. 2. The diagrams for the renormalization of the random hopping amplitude from the gauge fluctuations.

and the system is a nFL metal with finite BCS coupling in the IR. This is consistent with our result from solving the linearized gap equation. In particular, for $x \to 1/2$ (formally at $N \gg M$) the $\bar{c}$ dependence in (19) can be dropped. Indeed we find in this case Eq. (19) for the pairing QCP has the same asymptotic behavior as that of Eq. (16) of the main text, which is

$$M > \sqrt{2N}. \tag{21}$$

As was pointed out in Ref. 5, the RG formulation of the pairing problem also provides a clear interpretation of the KT scaling behavior[3]. At large $MN$, there are two fixed points for $\lambda$, one stable and the other unstable. At the critical value $M_{cr} = 8/[\alpha(x)\bar{c}^{1-2x}(1-2x)]$, these two critical points merge into one at $\lambda_{**} = (1-2x)\pi M_{cr}/2$. It is exactly the merger of two critical points that accounts for the KT scaling behavior near the critical point of e.g., the classical 2d XY model.[9] Here the KT scaling behavior occurs at $T = 0$ near a *quantum-critical* point.

## IV. CONFINEMENT OF THE RANDOM COMPACT GAUGE THEORY

In Ref. 10, the authors studied a random compact gauge theory similar to the random Yukawa theory we study[11], given by the Hamiltonian

$$H = \frac{1}{(MN)^{1/2}} \sum_{ij}^{N} \sum_{\alpha\beta}^{M} t_{\alpha\beta} e^{iA_{ij}} c^\dagger_{i\alpha} c_{j\beta} + \frac{g}{2} \sum_{ij}^{N} E^2_{ij}, \tag{22}$$

where $E_{ij}$ is the electric field conjugate to $A_{ij}$. The theory is invariant under the gauge transformation $A_{ij} \to A_{ij} + \theta_i - \theta_j$ and $c^\dagger_{i\alpha} \to c^\dagger_{i\alpha} e^{i\theta_i}$. One can also include a $A_0$ component, but since it couples to fermions diagonally with $i = j$, their effects are parametrically smaller than $A_{ij}$ and can be neglected. In fact, much of the normal state results obtained in Ref. 10 is very similar to what we presented in the main text.

In Ref. 10, it was assumed that the fermions screen the gauge field fluctuations and prevent a confinement transition. Under this assumption the gauge coupling was expanded to quadratic order as

$$e^{iA_{ij}} c^\dagger_i c_j \approx \left(1 + iA_{ij} - A^2_{ij}/2 + \cdots\right) c^\dagger_i c_j. \tag{23}$$

It was then obtained that the fermions displays nFL behavior, and the gauge fields are damped.

However, importantly, once the gauge field fluctuations are included *to all orders* of in (23), the theory does become confined at $T = 0$! Owing to the simple structure of this model, the confining phase can be exactly solved. To see this, we organize various gauge coupling vertices with various number of external photon lines as in Fig. 2. Summing the diagarms in each row, the non-perturbative effect of the gauge field fluctuations is a renormalization of the random (gauged) hopping amplitude $t_{\alpha\beta}$ with an exponential factor:

$$\begin{aligned} t_{\alpha\beta} \to t^*_{\alpha\beta} &\equiv t_{\alpha\beta} \exp\left(-\frac{D(\tau = 0_+)}{2}\right) \\ &= t_{\alpha\beta} \exp\left(-\frac{1}{2}\int \frac{d\Omega}{2\pi} D(\Omega)\right). \end{aligned} \tag{24}$$

where $D(\Omega)$ and $D(\tau)$ are the photon propagator, which in turn satisfies[10]

$$D(\Omega) = \frac{1}{\Omega^2/g + \Pi(\Omega) - \Pi(0)}, \text{ where}$$
$$\Pi(\Omega) = -\frac{2M}{N} t^{*2} \int \frac{d\omega}{2\pi} G(\omega) G(\omega+\Omega) \tag{25}$$

The *only* solution (at $T = 0$) of Eq. (24) is given by

$$t^*_{\alpha\beta} = 0, \text{ and } \Pi(\Omega) = 0, \tag{26}$$

To see this is a confined phase, note that the hopping amplitude $t^*_{\alpha\beta}$ is renormalized to zero, the fermions are confined to their site. More formally one can also compute the Wilson "loop" operator for the gauge field — in 0+1d it is computed at two end points in time, given by

$$\begin{aligned}\mathcal{W}(\tau) =& \langle e^{iA_{ij}(\tau) - iA_{ij}(0)} \rangle \\ =& \langle :e^{iA_{ij}(\tau)}: :e^{-iA_{ij}(0)}: \rangle \langle e^{iA_{ij}(0)} \rangle^2 \\ =& \exp\left[ g \int \frac{d\Omega}{2\pi} \frac{e^{i\Omega\tau}}{\Omega^2 + \epsilon^2} \right] \times \exp\left[ -g \int \frac{d\Omega}{2\pi} \frac{1}{\Omega^2 + \epsilon^2} \right],\end{aligned} \tag{27}$$

where we have added a small "Higgsed" mass to the gauge field to regularize the integral. Evaluating the integral, we get

$$\mathcal{W}(\tau) = \lim_{\epsilon \to 0} \exp\left[ \frac{g}{2\epsilon} (e^{-\epsilon\tau} - 1) \right] = e^{-g\tau/2}. \tag{28}$$

We see that the Wilson loop follows an "area law" decay[12], thus the gauge theory is in a confined phase.

---

[1] I thank Ilya Esterlis and Joerg Schmalian for discussions on this.
[2] I. Esterlis and J. Schmalian, Phys. Rev. B **100**, 115132 (2019).
[3] H. Wang, S. Raghu, and G. Torroba, Phys. Rev. **B95**, 165137 (2017), arXiv:1612.01971 [cond-mat.str-el].
[4] M. Metlitski, D. Mross, S. Sachdev, and T. Senthil, Phys. Rev. B **91**, 115111 (2015).
[5] S. Raghu, G. Torroba, and H. Wang, Phys. Rev. **B92**, 205104 (2015), arXiv:1507.06652 [cond-mat.str-el].
[6] We take the UV scale to be $\omega_0$, so we already have a full-fledged nFL scaling from the beginning. It is also possible to reproduce the nFL scaling behavior by running from the true UV scale of the theory — we leave it to future investigations.
[7] D. T. Son, Phys. Rev. D **59**, 094019 (1999).
[8] A. Fitzpatrick, S. Kachru, J. Kaplan, S. Raghu, G. Torroba, and H. Wang, Phys. Rev. **B92**, 045118 (2015), arXiv:1410.6814 [cond-mat.str-el].
[9] A. Altland and B. D. Simons, *Condensed matter field theory* (Cambridge University Press, 2010).
[10] A. A. Patel and S. Sachdev, Phys. Rev. B **98**, 125134 (2018).
[11] I thank A. Patel for stimulating discussions on this.
[12] E. Fradkin, *Field theories of condensed matter physics* (Cambridge University Press, 2013).
